# Supplementary material for: Learning Stable Classifiers by Transferring Unstable Features
Source: arXiv:2106.07847 source file (2022-06-27)
Supplement: Supplementary file 2 [file negative.tex]

\section{Negative social impact}
\label{app:negative}
